# Supplementary material for: Blockchain-based Secure Client Selection in Federated Learning
Source: arXiv:2205.05611 source file (2022-05-11)
Supplement: Supplementary file 1 [file appendix.tex]

% !TEX root = main.tex

\subsection{Verifiable Random Functions.}

%In our design, a verifiable random function (VRF) has been used for backbone miners to establish connections with other miners.
 Here, we present formal definitions of Verifiable Random Functions from \cite{dodis2005verifiable}. 
\begin{definition}
	A function family $F_{(\cdot)}(\cdot): \{0,1\}^\ell \rightarrow \{0,1\}^{\ell_{vrf}}$ is a family of VRFs if there exist algorithms $(\Gen,\Prove,\Verify)$ such that:
		\begin{itemize}
			\item The algorithm $\Gen$ takes as input a security parameter $1^\kappa$ and outputs a key pair $(\SK,\PK)$.
			\item The algorithm $\Prove$ takes as input a private key $\SK$, a string $x$, and outputs a pair $(F_{\SK}(x),\pi_{\SK}(x))$.
			\item The algorithm $\Verify$ takes as input a public key $\PK$, a string $x$, an output $\sigma$, a proof $\pi_{\SK}(x)$ and verifies that $\sigma = F_{\SK}(x)$ using the proof $\pi_{\SK}(x)$. It output $1$ if $y$ is valid and $0$ otherwise. 
		\end{itemize}
	Additionally, we require the following properties:
	\begin{enumerate}
		\item \textbf{Uniqueness.}  No values $(\PK,x,\sigma,\sigma',\pi_{\SK}(x),\pi_{\SK}(x)')$ can satisfy both
		$$\Verify_{\PK}(x,\sigma,\pi_{\SK}(x))=1 \text{ and } \Verify_{\PK}(x,\sigma',\pi_{\SK}(x)')=1$$
		unless $\sigma = \sigma'$
		\item \textbf{Provability.} If $\sigma,\pi_{\SK}(x) \gets \Prove_{\SK}(x)$, then $\Verify_{\PK}(x,\sigma,\pi_{\SK}(x))=1$.
		\item \textbf{Pseudorandomness.} For all \PPT adversary $\cA = (\cA_E,\cA_J)$, which runs for a total of $s(\kappa)$ steps when its first input is $1^\kappa$, and does not query the oracle on $x$, we have
		$$\Pr\left[		
		\begin{array}{l|l}
		(\PK,\SK)\leftarrow \Gen(1^\secp);\\
		(x,st) \gets \cA_E^{\Prove_{\SK}(\cdot)};&\\
		y_0 := F_{\SK}(x); 
		y_1 \gets \{0,1\}^{\ell_{vrf}};& b = b'\\
		b \gets \{0,1\};\\
		b' \gets  \cA_j^{\Prove_{\SK}(\cdot)}(y_b,st)&
		\end{array}
		\right] \le \frac{1}{2}\negl(\secp)$$
	\end{enumerate}
\end{definition}

\subsection{Chernoff bounds}

\begin{lemma}
	Suppose $\{X_i: i \in [n]\}$ are independent and identically distributed Bernoulli random variables with $\Pr[X_i = 1] = \mu$, for all $i \in [n]$. Then, for any $\varepsilon > 0$, we have
	\begin{align*}
		\Pr[\sum_{i=1}^n X_i \le (1-\varepsilon)n\mu] \le e ^{-\varepsilon^2n\mu/2} \\
		\Pr[\sum_{i=1}^n X_i \ge (1+\varepsilon)n\mu] \le e ^{-\varepsilon^2n\mu/3}
	\end{align*}
\end{lemma}
